# Supplementary material for: Learning Neural Parsers with Deterministic Differentiable Imitation Learning
Source: arXiv:1806.07822 source file (2018-09-19)
Supplement: Supplementary file 1 [file supplementary.tex]

\documentclass{article}

\usepackage{corl_2018}
\usepackage{multicol}
\usepackage{float}
\usepackage{mathtools}
\usepackage{amsfonts}
\usepackage{booktabs}
\usepackage{epstopdf}
\usepackage{svg}
\usepackage{multirow}
\usepackage{enumitem}
\usepackage{grffile}
\usepackage[noend]{algpseudocode}
\usepackage{algorithm}
\usepackage{amsmath}
\usepackage{amsfonts}

\title{Supplementary material for Learning Neural Parsers with Deterministic Differentiable Imitation Learning}

\author{
  David S.~Hippocampus\\
  Department of Electrical Engineering and Computer Sciences\\
  University of California Berkeley 
  United States\\
  \texttt{hippo@berkeley.edu} \\
}

\begin{document}
\maketitle

\input{supplementary_body.tex}

\bibliography{references} 

\end{document}
